# Supplementary material for: Collaborative Visual Place Recognition
Source: arXiv:2310.05541 source file (2023-10-09)
Supplement: Supplementary file 1 [file Appendix.tex]

% \section*{TF-VPR Supplement}\label{app}

% \section*{Appendix}
\setcounter{section}{0}
\setcounter{figure}{0}
\setcounter{table}{0}
\providecommand{\titlevariable}{TF-VPR}

In the supplement material, we provide more visualizations and analyses. More specifically, we show: (1) the visualizations of our dataset and the agent's trajectory; (2) the computation time of different methods in the training and inference phases; (3) the qualitative results of the query and its corresponding retrieved positives.

\section{Dataset}
% \textbf{Pointcloud dataset}\cc{Assigned to Dingli}

\textbf{Point cloud dataset.}
2D simulated point cloud dataset: we simulate 2D point clouds captured by the mobile agents equipped with virtual Lidar sensors. Specifically, we first create the 2D environment, represented as a binary image with the resolution of $1024\times 1024$, as shown in Fig.~\ref{fig:pointcloud}. The white and blue pixels correspond to the free space and the obstacles, respectively. Given the 2D environment, we interactively sample the trajectory of the mobile agent. For each sampled pose, the points in the simulated point clouds are the intersection points between laser beams and the obstacle boundaries. In our experiments, the virtual Lidar sensor has the field-of-view of $360^{\circ}$ with the angular resolution of $1^{\circ}$ (equivalently, each point cloud has 256 points). We created 18 trajectories sampled from 10 environments. Each trajectory contains 2048 poses. On average, the rotational and translation perturbation between two consecutive poses are $\pm 10^{\circ}$ and $\pm 
9.60\, pixel$, respectively. 

\begin{figure*}[t]
    \centering {\includegraphics[trim={0.7cm 12cm 1.5cm 0.5cm},clip,width=1\textwidth
    ]{figs/Env_figs/dataset_pc.pdf}} \quad
    \vspace{-4mm}
    \caption{\textbf{Qualitative demonstrations of the 2D point cloud dataset}. The upper-left image shows one of the trajectories in the dataset. Each point on the trajectory is assigned with color to represent its timestamp. The arrows on each point indicate their orientations. The point clouds captured at several trajectory points are visualized.}
    \label{fig:pointcloud}
\end{figure*}

\textbf{Habitat-Sim dataset} We collected the photo-realistic simulated images in the habitat-sim~\cite{savva2019habitat} simulator using the Gibson~\cite{xiazamirhe2018gibsonenv} dataset. The RGB images were captured by a virtual 360 camera mounted on a virtual robot in the environment. The robot moved according to the random exploration strategy. In total, we collected more than 10k images in 18 scenes. Fig~\ref{fig:goffs} shows some examples of images and the robot trajectories.

\begin{figure*}[t]
    \centering {\includegraphics[trim={0.7cm 15cm 0.5cm 0.5cm},clip,width=1\textwidth
    ]{figs/Env_figs/dataset_goffs.pdf}} \quad
    \vspace{-9mm}
    \caption{\textbf{Qualitative demonstrations of the  photorealistic RGB dataset}. The legend follows Fig.~\ref{fig:pointcloud}}
    \label{fig:goffs}
\end{figure*}

\textbf{Real-world RGB dataset.}
We collected the real RGB dataset captured by Gopro MAX, a dual-lens 360 camera with GPS recording. The GoPro camera was mounted on the top of the driving vehicle. Our dataset collection area selected an urban zone containing eight townhouse blocks. As shown in Fig.~\ref{fig:real-rgb}, we collected three different trajectories from the same start points. All trajectories contain visits to the same intersections for the loop closure detection. We designed three different actions for the same intersection: turn left, turn right and go ahead, with two opposite driving directions. Except for a few intersections due to traffic reasons, most intersections contain at least two kinds of actions with different driving directions. 

\begin{figure*}[t]
    \centering {\includegraphics[trim={0.7cm 13cm 0.5cm 0.5cm},clip,width=1.0\textwidth
    ]{figs/Env_figs/dataset_scene1.pdf}} \quad
    \vspace{-8mm}
    \caption{\textbf{Qualitative demonstrations of the collected real-world RGB dataset}. The legend follows Fig.~\ref{fig:pointcloud}}
    \label{fig:real-rgb}
\end{figure*}

% \clearpage
\section{Computation Time}

We report computation time in both training and inference phases in Table~\ref{Time_table} with $hh:mm:ss$ format. Regarding the training phase, the computation includes network optimization and label refurbishment. Compared with other learnable or hand-crafted methods, our method only needs to consume more time for training, but does not introduce an extra burden for inference. The more time consuming in training is because of label refurbishment which requires feature space neighborhoods as well as pairwise geometric verification. Note that compared to the brute-force pairwise geometric verification, our training is more affordable thanks to the elaborate temporal and feature neighborhoods mining.

% Please add the following required packages to your document preamble:
% \usepackage{multirow}

\begin{table}[ht!]
\resizebox{1\linewidth}{!}{
\begin{tabular}{|c|cc|cccccc|clcllllclllll|}
\hline
\multirow{2}{*}{Dataset} & \multicolumn{2}{c|}{Point Cloud} & \multicolumn{6}{c|}{Habitat Scene }  & \multicolumn{13}{c|}{Real RGB} \\
\cline{2-22}   & \multicolumn{2}{c|}{Scene} & \multicolumn{2}{c|}{Goffs}   & \multicolumn{2}{c|}{Micanopy}  & \multicolumn{2}{c|}{Spotswood}   & \multicolumn{2}{c|}{Scene 1}   & \multicolumn{11}{c|}{Scene 2}    \\ \hline
Metric                   & \multicolumn{1}{c|}{Train}        & Eval.       & \multicolumn{1}{c|}{Train} & \multicolumn{1}{c|}{Eval.} & \multicolumn{1}{c|}{Train} & \multicolumn{1}{c|}{Eval.} & \multicolumn{1}{c|}{Train} & Eval. & \multicolumn{1}{c|}{Train}     & \multicolumn{1}{l|}{Eval.} & \multicolumn{5}{c|}{Train}     & \multicolumn{6}{c|}{Eval.}  \\ \hline
SPTM                     & \multicolumn{1}{c|}{0:49:14}             &    0:00:12            &  \multicolumn{1}{c|}{0:58:34}      & \multicolumn{1}{c|}{0:13:23}         & \multicolumn{1}{c|}{0:34:57}      & \multicolumn{1}{c|}{0:07:29}         & \multicolumn{1}{c|}{1:28:12}      &   0:09:13       & \multicolumn{1}{c|}{2:21:36}          & \multicolumn{1}{l|}{0:05:59}         & \multicolumn{5}{c|}{0:40:04}          & \multicolumn{6}{c|}{0:14:33}          \\
PCL                      & \multicolumn{1}{c|}{N/A}          &   N/A             & \multicolumn{1}{c|}{0:15:45}      & \multicolumn{1}{c|}{0:01:20}         & \multicolumn{1}{c|}{0:17:32}      & \multicolumn{1}{c|}{0:01:15}         & \multicolumn{1}{c|}{0:19:24}      &      0:01:12    & \multicolumn{1}{c|}{0:28:55}          & \multicolumn{1}{l|}{0:09:29}         & \multicolumn{5}{c|}{0:13:25}          & \multicolumn{6}{c|}{0:07:19}          \\
Ours                     & \multicolumn{1}{c|}{5:38:12}             &    0:00:06            & \multicolumn{1}{c|}{21:01:06}      & \multicolumn{1}{c|}{0:09:46}         & \multicolumn{1}{c|}{12:38:49}      &  \multicolumn{1}{c|}{0:05:33}         & \multicolumn{1}{c|}{15:03:50}      &  0:06:28        & \multicolumn{1}{c|}{3:33:46} & \multicolumn{1}{l|}{0:04:16}         & \multicolumn{5}{c|}{8:35:10} & \multicolumn{6}{c|}{0:09:54} \\ \hline
VLAD                     & \multicolumn{1}{c|}{N/A}          &  N/A              & \multicolumn{1}{c|}{0:02:14}      & \multicolumn{1}{c|}{0:02:39}         & \multicolumn{1}{c|}{0:05:29}      & \multicolumn{1}{c|}{0:04:31}         & \multicolumn{1}{c|}{0:03:46}      &  0:04:09        & \multicolumn{1}{c|}{0:12:07}          & \multicolumn{1}{l|}{2:44:50}         & \multicolumn{5}{c|}{0:14:19}          & \multicolumn{6}{c|}{0:52:09}          \\
NetVLAD               & \multicolumn{1}{c|}{3:57:09}             &      0:00:27          & \multicolumn{1}{c|}{0:54:04}      & \multicolumn{1}{c|}{0:06:42}         & \multicolumn{1}{c|}{:0:31:27}      & \multicolumn{1}{c|}{0:04:17}         & \multicolumn{1}{c|}{0:40:08}      &    0:05:01      & \multicolumn{1}{c|}{1:00:06}          & \multicolumn{1}{l|}{0:14:41}         & \multicolumn{5}{c|}{0:22:41}          & \multicolumn{6}{c|}{0:04:16}          \\ \hline
Pair. Verif.  & \multicolumn{2}{c|}{46731:25:31} & \multicolumn{2}{c|}{6630:16:19}   & \multicolumn{2}{c|}{2294:31:07}  & \multicolumn{2}{c|}{2915:44:43}   & \multicolumn{2}{c|}{11083:40:57}   & \multicolumn{11}{c|}{5350:30:50}         \\ \hline
\end{tabular}
}   
\vspace{2mm}
\caption{\textbf{Training and inference time} of each method on three different datasets. Train represents the training time for one epoch. Eval. represents inference time. Pair. Verif. means pairwise verification method.}
\label{Time_table}
\end{table}

\section{Qualitative Comparisons}

We use our best performing network (CNN, VGG-16) trained completely on the point cloud, habitat scene, and real-world datasets, to extract point cloud or image representations for standard image retrieval methods. Fig. \ref{fig:query_pc} compares \titlevariable\, to the state-of-the-art point cloud representations. It shows our method outperforms SPTM by a large margin. SPTM can only retrieve the true positives from a similar orientation, whereas TF-VPR can retrieve neighbors regardless of its orientation. Fig.~\ref{fig:query_goffs} and \ref{fig:query_realrgb} compares \titlevariable\, to the state-of-the-art image representations. The upper part of both figures shows an example where our method can achieve a better recall rate on different datasets by a large margin. However, the lower part shows some difficult examples.
\vspace{-15mm}

\vspace{-15mm}
\clearpage

\clearpage
